# Supplementary material for: Hybrid Low-Power Wide-Area Mesh Network for IoT Applications
Source: arXiv:2006.12570 source file (2020-06-22)
Supplement: Supplementary file 1 [file appendix.tex]

\appendices
\section{Proof of the First Zonklar Equation}
\label{sec:appendix}
Appendix one text goes here.

% you can choose not to have a title for an appendix
% if you want by leaving the argument blank
\section{}
Appendix two text goes here.
